# Supplementary material for: Ray-Based Reflectance Model for Diffraction
Source: arXiv:1101.5490 source file (2011-01-28)
Supplement: Supplementary file 1 [file audio-appendix.tex]

% !TEX root = ./wbsdf-tog.tex

%\section*{WBSDF in Audio}

%For efficient rendering of sound, many techniques assume that high frequency sound waves can be modeled as rays. The two main diffraction models used in these geometric simulations are the Uniform Theory of Diffraction (UTD)~\cite{Kouyoumjian1974,Tsingos2001} and Biot--Tolstoy--Medwin (BTM) model~\cite{hothersall1991,Torres2001}. These techniques, which are often referred to as edge--diffraction, first search for diffracting edges and then create new sources at those positions. UTD based--methods scatter incoming sound beams in a cone around the edge, where the half--angle of the cone is determined by the angle that the ray hits the edge~\cite{Chandak2008,Rick2007}. They are often preferred because of efficiency, but are less accurate in lower frequencies. BTM is more accurate and is also applicable for non--geometric acoustics~\cite{Torres2001}, but is not applicable for interactive renderings due to its complexity.\\

The same formulation as the rendering equation exists for sound rendering and is called the room acoustic rendering equation~\cite{siltanen:1624}. The derivation for this room acoustic rendering equation is similar to section~\ref{sec:concept}. We therefore show that this BSDF is applicable for audio as well under an infinite speed assumption.\\
